# Supplementary material for: Machine Learning for Polymer Chemical Resistance to Organic Solvents
Source: arXiv:2509.05344 source file (2025-09-02)
Supplement: Supplementary file 1 [file Supporting_Information.pdf]

## Supporting Information

**Machine Learning for Polymer Chemical Resistance to Organic Solvents.**

Shogo Kunieda<sup>1</sup>, Mitsuru Yambe<sup>1</sup>, Hiromori Murashima<sup>1</sup>, Takeru Nakamura<sup>1</sup>, Toshiaki Shintani<sup>2</sup>,  
Hitoshi Kamijima<sup>2</sup>, Yoshihiro Hayashi<sup>3</sup>, Yosuke Hanawa<sup>1</sup> and Ryo Yoshida<sup>3,4,5</sup>

<sup>1</sup>SCREEN Holdings. Co., Ltd., Kyoto 612-8486, Japan.

<sup>2</sup>Research Institute of Systems Planning. Inc., Tokyo 150-0031, Japan.

<sup>3</sup>The Institute of Statistical Mathematics, Research Organization of Information and Systems, Tachikawa,  
Tokyo 190-8562, Japan.

<sup>4</sup>Graduate Institute for Advanced Studies, SOKENDAI, Tachikawa, Tokyo 190-8562, Japan.

<sup>5</sup>Advanced General Intelligence for Science Program (AGIS), RIKEN TRIP, Wako, Saitama 351-0198, Japan

\*kunieda@screen.co.jp, \*hanawa@screen.co.jp, \*yoshidar@ism.ac.jp

## Contents

|                                                                      |    |
|----------------------------------------------------------------------|----|
| 1. Chemical resistance dataset.....                                  | 2  |
| 2. Force field kernel mean descriptor.....                           | 9  |
| 3. Flory–Huggins $\chi$ parameter.....                               | 10 |
| 4. LOOCV ROC-AUC on chemical resistance classification model .....   | 11 |
| 5. Validation results of the crystallinity classification model..... | 14 |
| 6. Distribution of solvent properties.....                           | 15 |
| 7. $\chi$ Parameter Distribution .....                               | 16 |
| 8. References.....                                                   | 19 |

## 1. Chemical resistance dataset

In this study, to develop a machine learning model for predicting the chemical resistance of polymers against organic solvents, we constructed a custom dataset by collecting and integrating polymer–solvent evaluation data from various chemical resistance charts published by manufacturers.<sup>1–6</sup>

The evaluation criteria used by different manufacturers vary significantly, including letter grades, symbolic notations, and qualitative expressions, making direct standardization difficult. To address this, we adopted a conservative annotation strategy: only polymer–solvent combinations consistently labeled as “resistant” across all sources were assigned a resistance label of 0 (resistant), while any combination labeled as “non-resistant” in at least one source was assigned a label of 1 (non-resistant). This approach enabled us to integrate data from multiple references without inconsistency and convert it into a binary classification format suitable for machine learning.

Based on this annotation policy, chemical resistance labels were assigned to 2,231 polymer–solvent pairs involving 27 polymers and 132 organic solvents. Each polymer was further annotated with a crystallinity binary label according to conventional classifications. Specifically, for thermoplastic polymers, those generally recognized as crystalline were labeled as 1, and those considered amorphous were labeled as 0. As a result, 18 polymers were classified as crystalline and 9 as amorphous.

To visualize variation in chemical resistance, Figure S1 shows the proportion of non-resistant labels (label 1) for each polymer. The polymers are displayed along the x-axis in ascending order of resistance (i.e., in descending order of label 1 proportion), and the y-axis indicates the proportion of non-resistant cases. This histogram format provides a visual representation of how polymer structure and crystallinity influence chemical resistance.

Given the large number of solvents (132), it is challenging to directly evaluate resistance trends across individual solvents. Therefore, for the purpose of model validation, we introduced solvent cluster classification to enable Leave-One-Group-Out Cross Validation (LOGOCV). Because the number of resistance evaluations per solvent varies, we considered both class imbalance and data quantity when clustering solvents into 10 groups. These clusters were sorted by the proportion of non-resistant labels: Cluster 1 includes solvents with high solubility (low resistance), and Cluster 10 includes those with low solubility (high resistance), thereby reflecting a gradient of chemical resistance across all solvents.

Figure S2 presents a two-dimensional matrix visualization for each solvent cluster, where solvents are shown on the y-axis and polymers on the x-axis. Resistance outcomes are color-coded: green for resistant (label 0) and red for non-resistant (label 1), enabling intuitive understanding of resistance patterns across polymer–solvent combinations.

Chemical resistance data, total number : 2,231, solvent : 132, polymer : 27

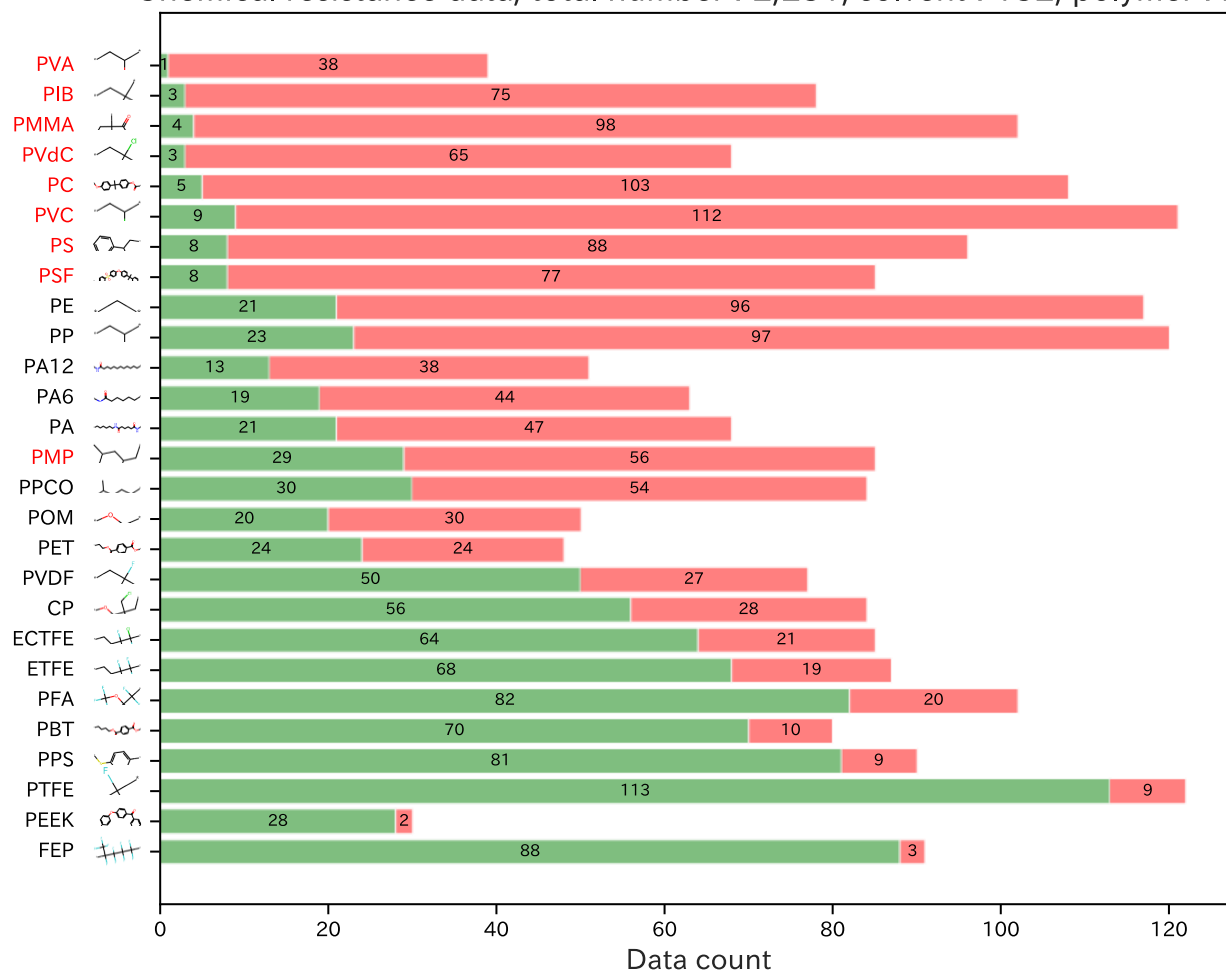

Figure S1: Distribution of chemical resistance data for each polymer. The y-axis lists abbreviations for the 27 polymers, while the x-axis shows the number of chemical resistance data points. Green and red bars represent the number of resistant and non-resistant cases, respectively. Polymers on the y-axis are ordered from top to bottom according to the proportion of non-resistant cases, meaning polymers with lower chemical resistance appear at the top. Amorphous and crystalline polymers are indicated in red and black, respectively.

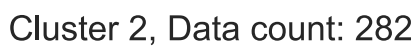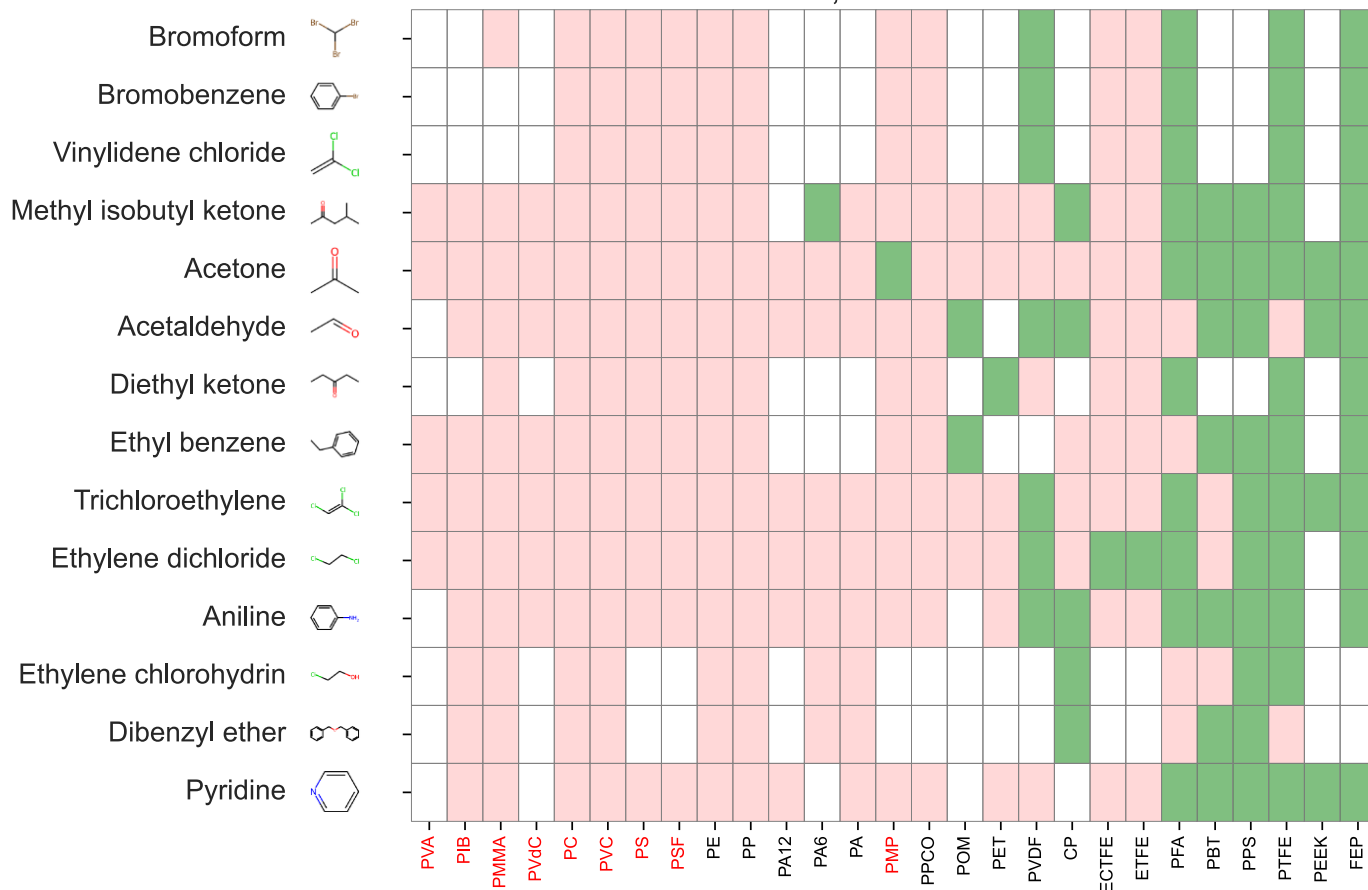

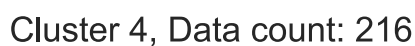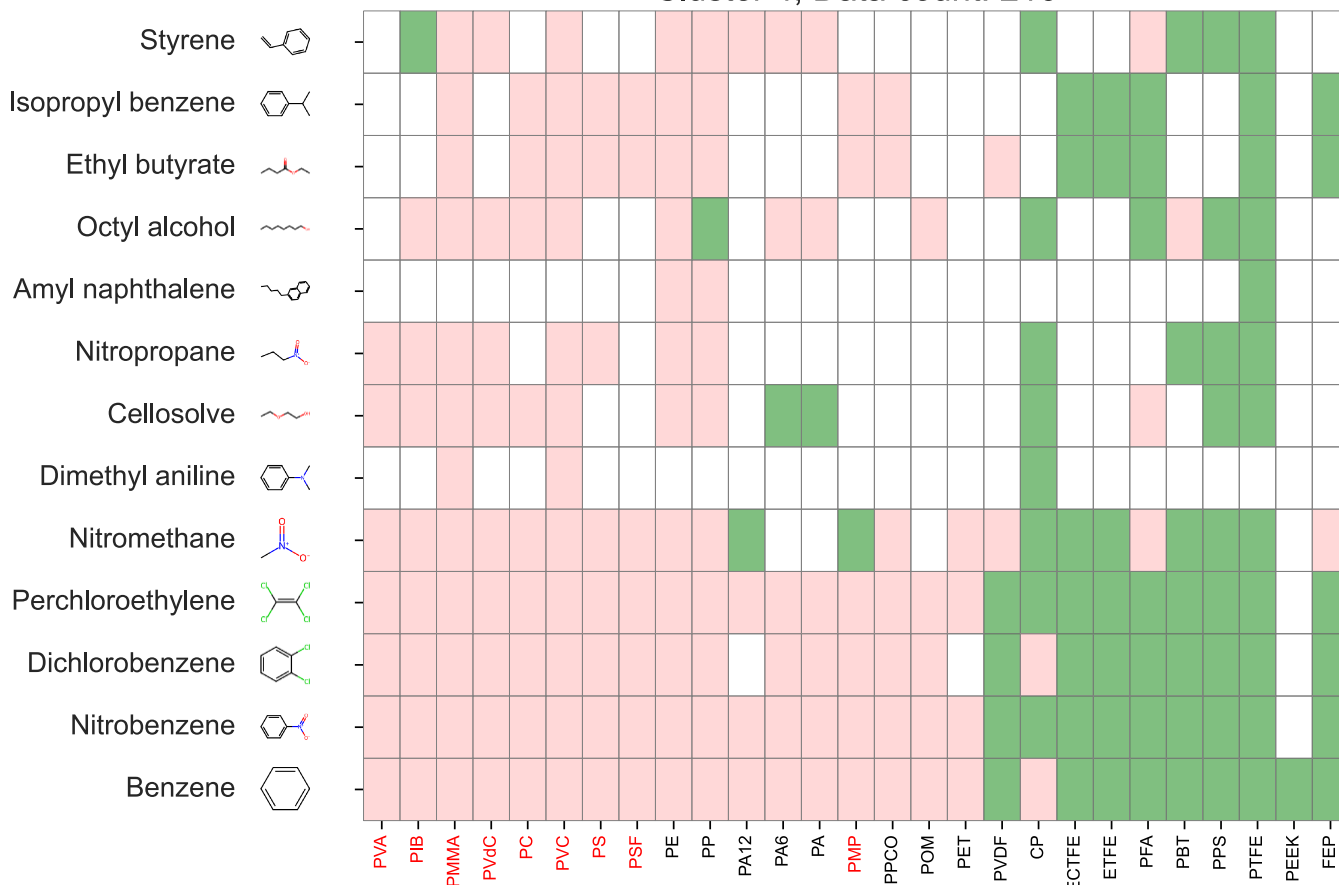

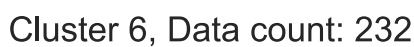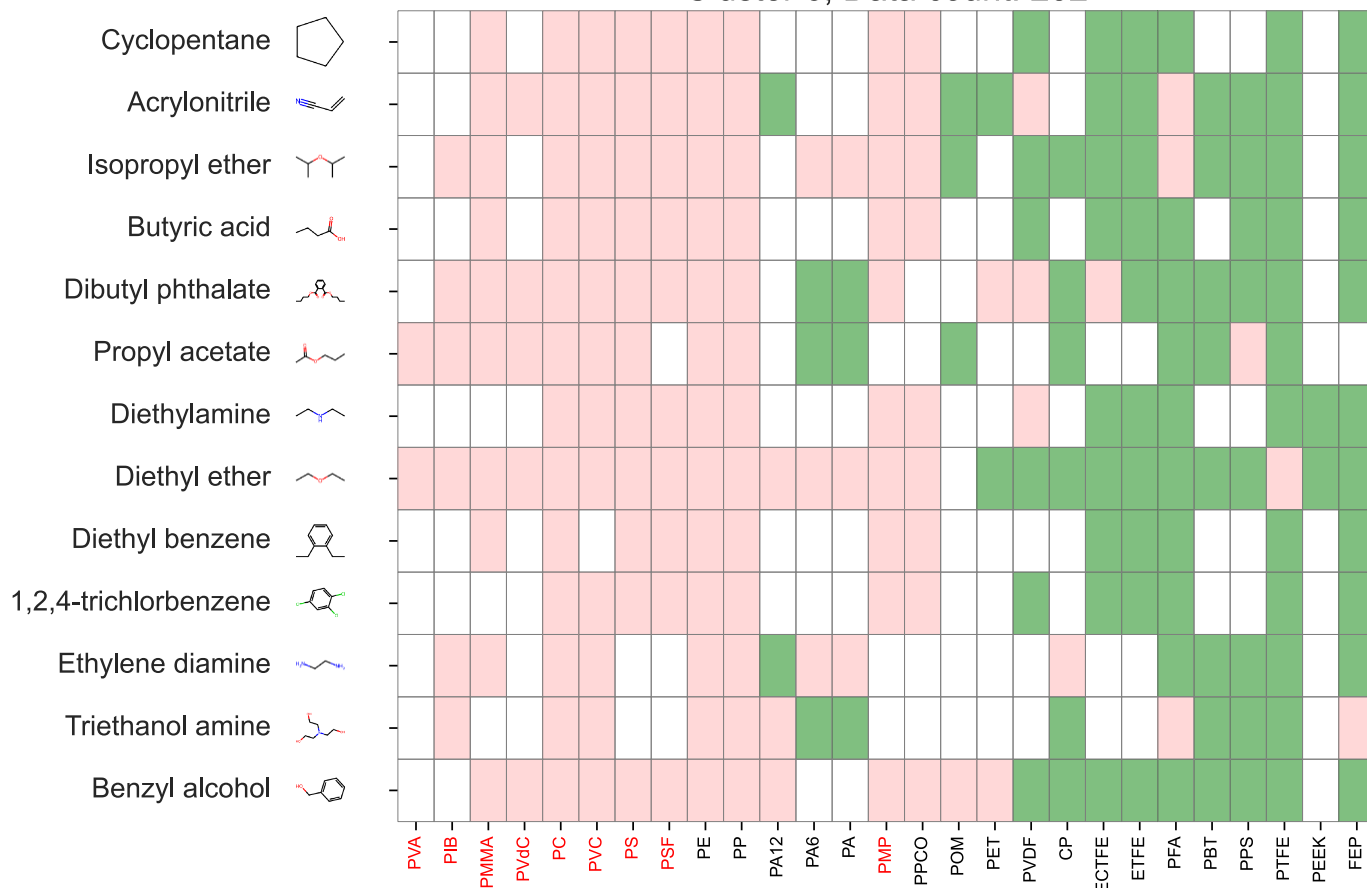

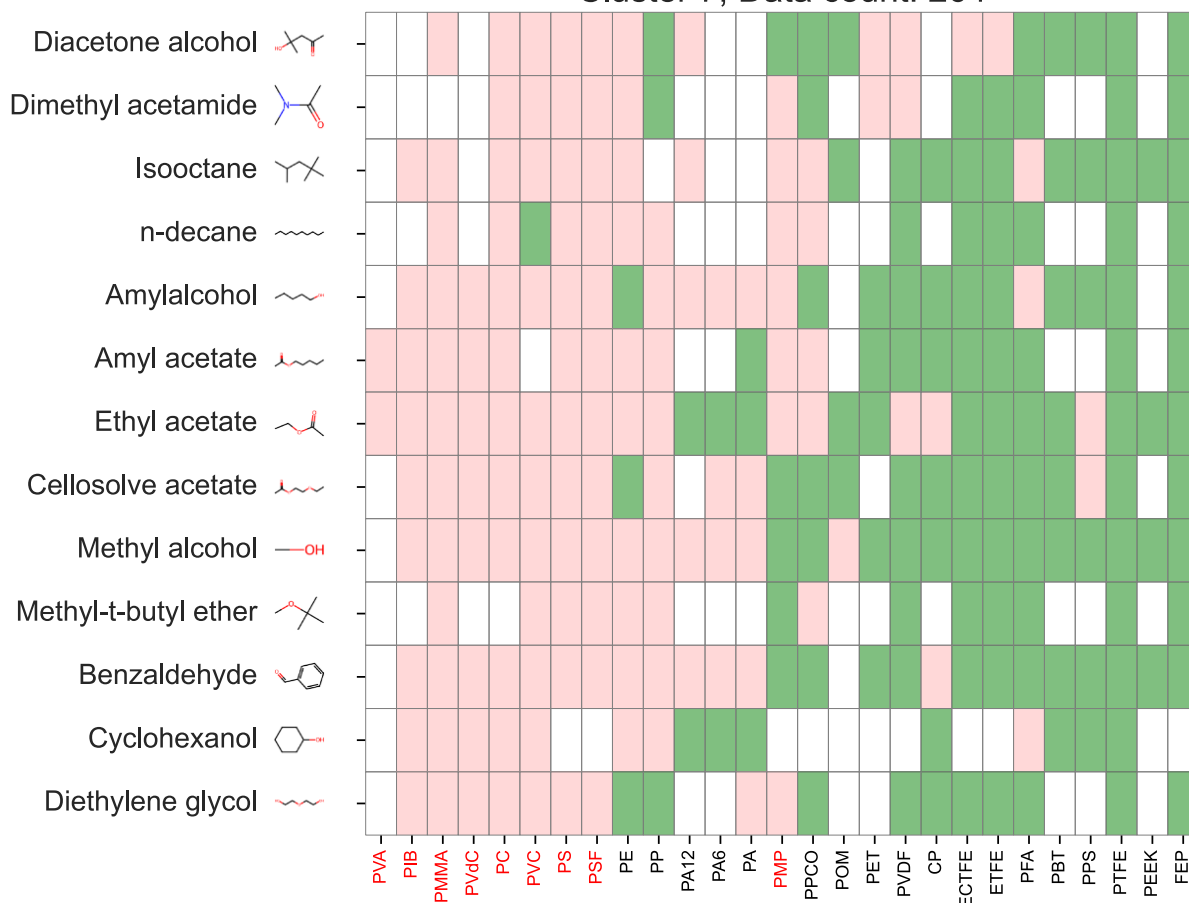

Cluster 8, Data count: 242

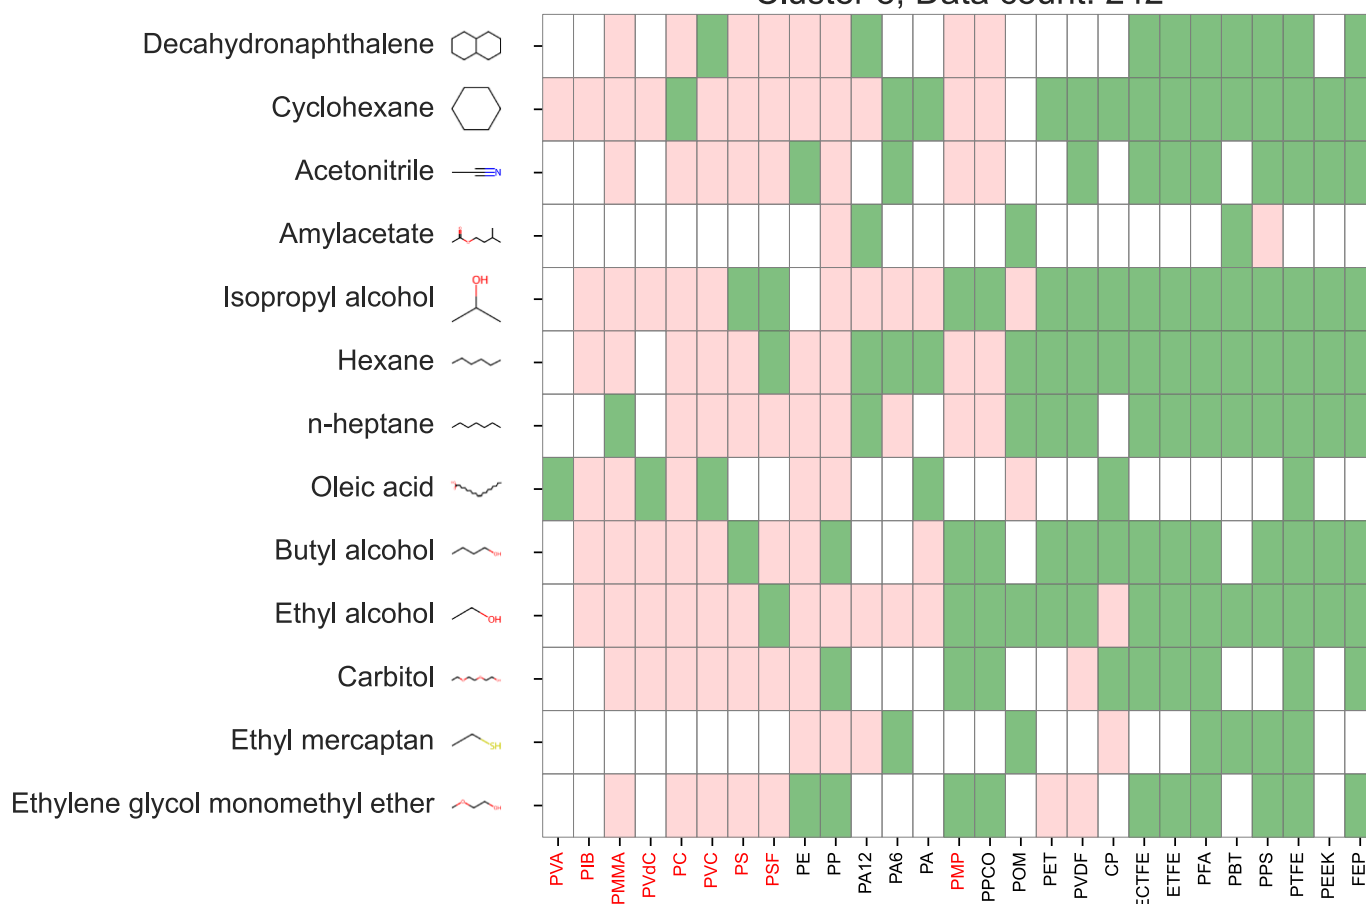

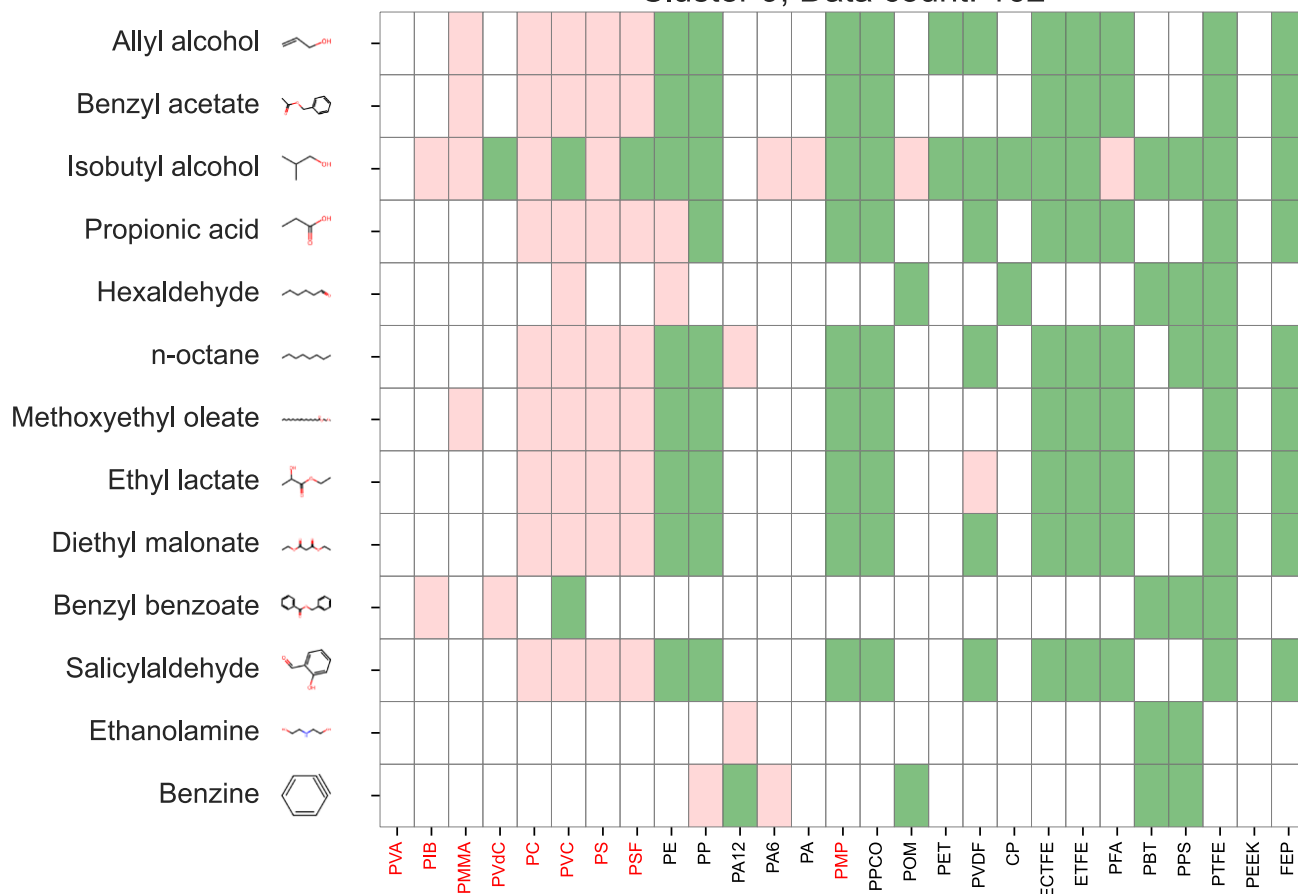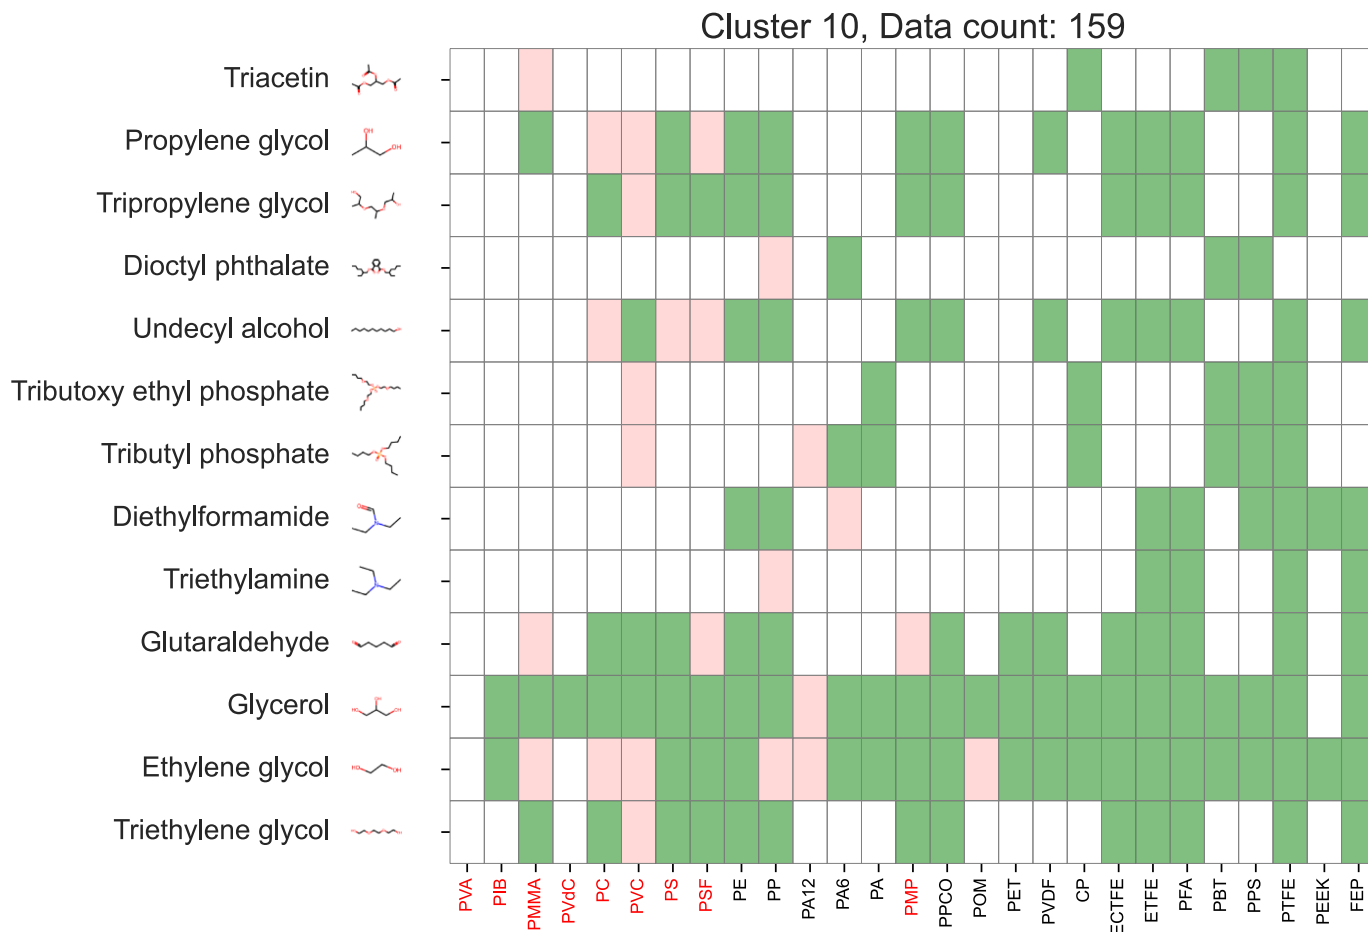



Figure S2: Chemical resistance data by solvent cluster. The y-axis lists organic solvents, sorted from top to bottom in descending order of the proportion of non-resistant cases. The x-axis represents polymer types, sorted from left to right in descending order of the proportion of non-resistant cases. Amorphous and crystalline polymers are indicated in red and black, respectively.

## 2. Force field kernel mean descriptor

In this study, we constructed structural descriptors for polymers and solvents by statistically vectorizing the distribution of force field parameters assigned to molecular structures.<sup>7</sup> Specifically, we applied kernel mean embedding to the distributions of each force field parameter to create fixed-length vectors, which we refer to as Force-Field Kernel Mean (FFKM) descriptors. This approach enables the generation of high-dimensional, unified descriptors that are independent of molecular size or structural complexity.

### List of Force Field Parameters Used

The following ten parameters were extracted, corresponding to atoms, bonds, angles, and dihedrals. All parameters are derived from the GAFF2 force field and were selected for their well-defined physical meaning:

| Target Type | Name                  | Description                                                     |
|-------------|-----------------------|-----------------------------------------------------------------|
| Atom        | mass                  | Atomic mass                                                     |
| Atom        | $\sigma$              | van der Waals equilibrium distance                              |
| Atom        | $\epsilon$            | Depth of van der Waals potential well                           |
| Atom        | charge                | Atomic charge (Gasteiger model)                                 |
| Bond        | $r_0$                 | Bond equilibrium length                                         |
| Bond        | $K_{\text{bond}}$     | Bond stretching force constant                                  |
| Bond        | polar                 | Bond polarity (absolute charge difference between bonded atoms) |
| Angle       | $\theta_0$            | Bond angle equilibrium value                                    |
| Angle       | $K_{\text{angle}}$    | Angle bending force constant (angular stiffness)                |
| Dihedral    | $K_{\text{dihedral}}$ | Dihedral rotational barrier height                              |

Note: The "polar" descriptor was additionally defined to quantify the polarity of atomic pairs.

### Vectorization Method and Implementation

For each descriptor, all corresponding parameter values in a molecule were extracted, and kernel density estimation (KDE) was applied using a Gaussian kernel. The resulting smoothed probability density function was evaluated over a predefined grid to obtain a fixed-dimensional vector representation for each descriptor.

Kernel mean embedding is defined by the following equation:

$$m(X) = \frac{1}{n} \sum_{i=1}^n k\left(\frac{X - X_i}{h}\right)$$

Here,

$X_i$  represents the descriptor values within a molecule (e.g., atomic charge or bond length),  $k(\cdot)$  is the kernel function based on the standard normal distribution, and  $h$  denotes the bandwidth (smoothing parameter). This equation corresponds to the method of constructing a continuous density function  $m(X)$  by convolving a Gaussian kernel over the histogram of descriptor values. The resulting density function was evaluated on a predefined grid to generate numerical sequences, which were used as descriptor vectors:

mass: Represented as a 10-dimensional vector corresponding to 10 representative elements (H, C, N, O, ...)

Other 9 descriptors: Each divided into 20 grid intervals and represented as 20-dimensional vectors

As a result, every molecule was assigned a fixed-length 190-dimensional vector ( $10 + 9 \times 20$ ). Descriptor generation was automated using the Python library RadonPy.<sup>8</sup>

### 3. Flory–Huggins $\chi$ parameter

In this study, we used COSMOtherm (Version 23), a software package based on the COSMO-RS (Conductor-like Screening Model for Real Solvents) method, to calculate thermodynamic properties of chemical compounds. By inputting molecular structural information (e.g., SMILES format), COSMOtherm can rapidly and accurately compute various properties, including solubility, activity coefficients, vapor pressure, and the Flory–Huggins  $\chi$  parameter for polymer–solvent systems.

COSMO-RS predicts the free energy and activity coefficients of mixtures using statistical thermodynamics, based on the polarity distribution (surface charge density) of molecular surfaces calculated via quantum chemical methods. Compared to traditional Hansen solubility parameters (HSP), COSMO-RS offers greater generality and is applicable to arbitrary polymer structures and solvents, making it a powerful tool in materials informatics.

TURBOMOLE (V7.8) was used to generate COSMO files,<sup>9</sup> and COSMOtherm (Version 23) was used to calculate the  $\chi$  parameters.<sup>10</sup> Initial 3D molecular structures were generated using the “Converts a Daylight SMILES text property to a molecule” module in Pipeline Pilot, followed by geometry optimization at various levels of theory. For polymers, structures containing 1 to 3 repeating units were created, with both chain ends capped by methyl groups.

After generating the COSMO files, we executed the COSMOmeso module in COSMOtherm, which calculates  $\chi$  parameters using activity coefficients derived from the COSMO files. Based on Flory–Huggins theory, the  $\chi$  parameter is defined as follows for a given set of activity coefficients, temperature, and mixing conditions:

$$\ln \gamma_s = \ln \left( \frac{\Phi_s}{x_s} \right) + \left( 1 - \frac{1}{r} \right) \Phi_p + \chi_{sp}(T) \Phi_p^2 \quad \cdot \cdot \cdot (1)$$

$$\ln \gamma_p = \ln \left( \frac{\Phi_p}{x_p} \right) + (1 - r) \Phi_s + \chi_{sp}(T) \Phi_s^2 \quad \cdot \cdot \cdot (2)$$

$$r = \frac{V_p}{V_s} \quad \cdot \cdot \cdot (3)$$

Here,  $\gamma_i$  denotes the activity coefficient of component,  $\chi_i(T)$  is the Flory–Huggins interaction parameter,  $\Phi_i$  is the volume fraction,  $x_i$  is the mole fraction, and  $r$  represents the reference volume ratio. In polymer–solvent systems,  $V_s$  and  $V_p$  refer to the molecular volumes of the solvent and the polymer repeating unit, respectively. In this study, all  $\chi$  parameters were estimated using Equation (3).

To achieve a volume fraction of 50:50 in polymer–solvent systems,  $\chi$  parameters were calculated twice and averaged accordingly.<sup>11</sup>

The quantum chemical calculation settings used for  $\chi$  parameter estimation in this study were as follows:

- **Geometry optimization:** xTB\_def-SV(P)
- **COSMO file generation:** B3LYP-def2-SVP (TURBOMOLE)

Using the above protocol,  $\chi$  parameters were calculated for all 2,231 polymer–solvent pairs included in the dataset.

For polymer–solvent pairs not covered in the dataset, predicted  $\chi$  values were generated using a random forest regression model trained on the 2,231 computed  $\chi$  data points. Ten-fold cross-validation of the random forest model yielded a performance of  $R^2 = 0.805 \pm 0.147$ ,  $MAE = 0.199 \pm 0.032$ ,  $RMSE = 0.479 \pm 0.265$ . The training performance on the full dataset was  $R^2 = 0.999$ ,  $MAE = 0.0188$ ,  $RMSE = 0.0274$ .

## 4. LOOCV ROC-AUC on chemical resistance classification model

This section summarizes the validation performance described in Section 3.1 of the main text. Leave-One-Group-Out Cross-Validation was conducted for 27 polymers and 10 solvent clusters. The classification threshold for predicted chemical resistance probability was set to 0.9.

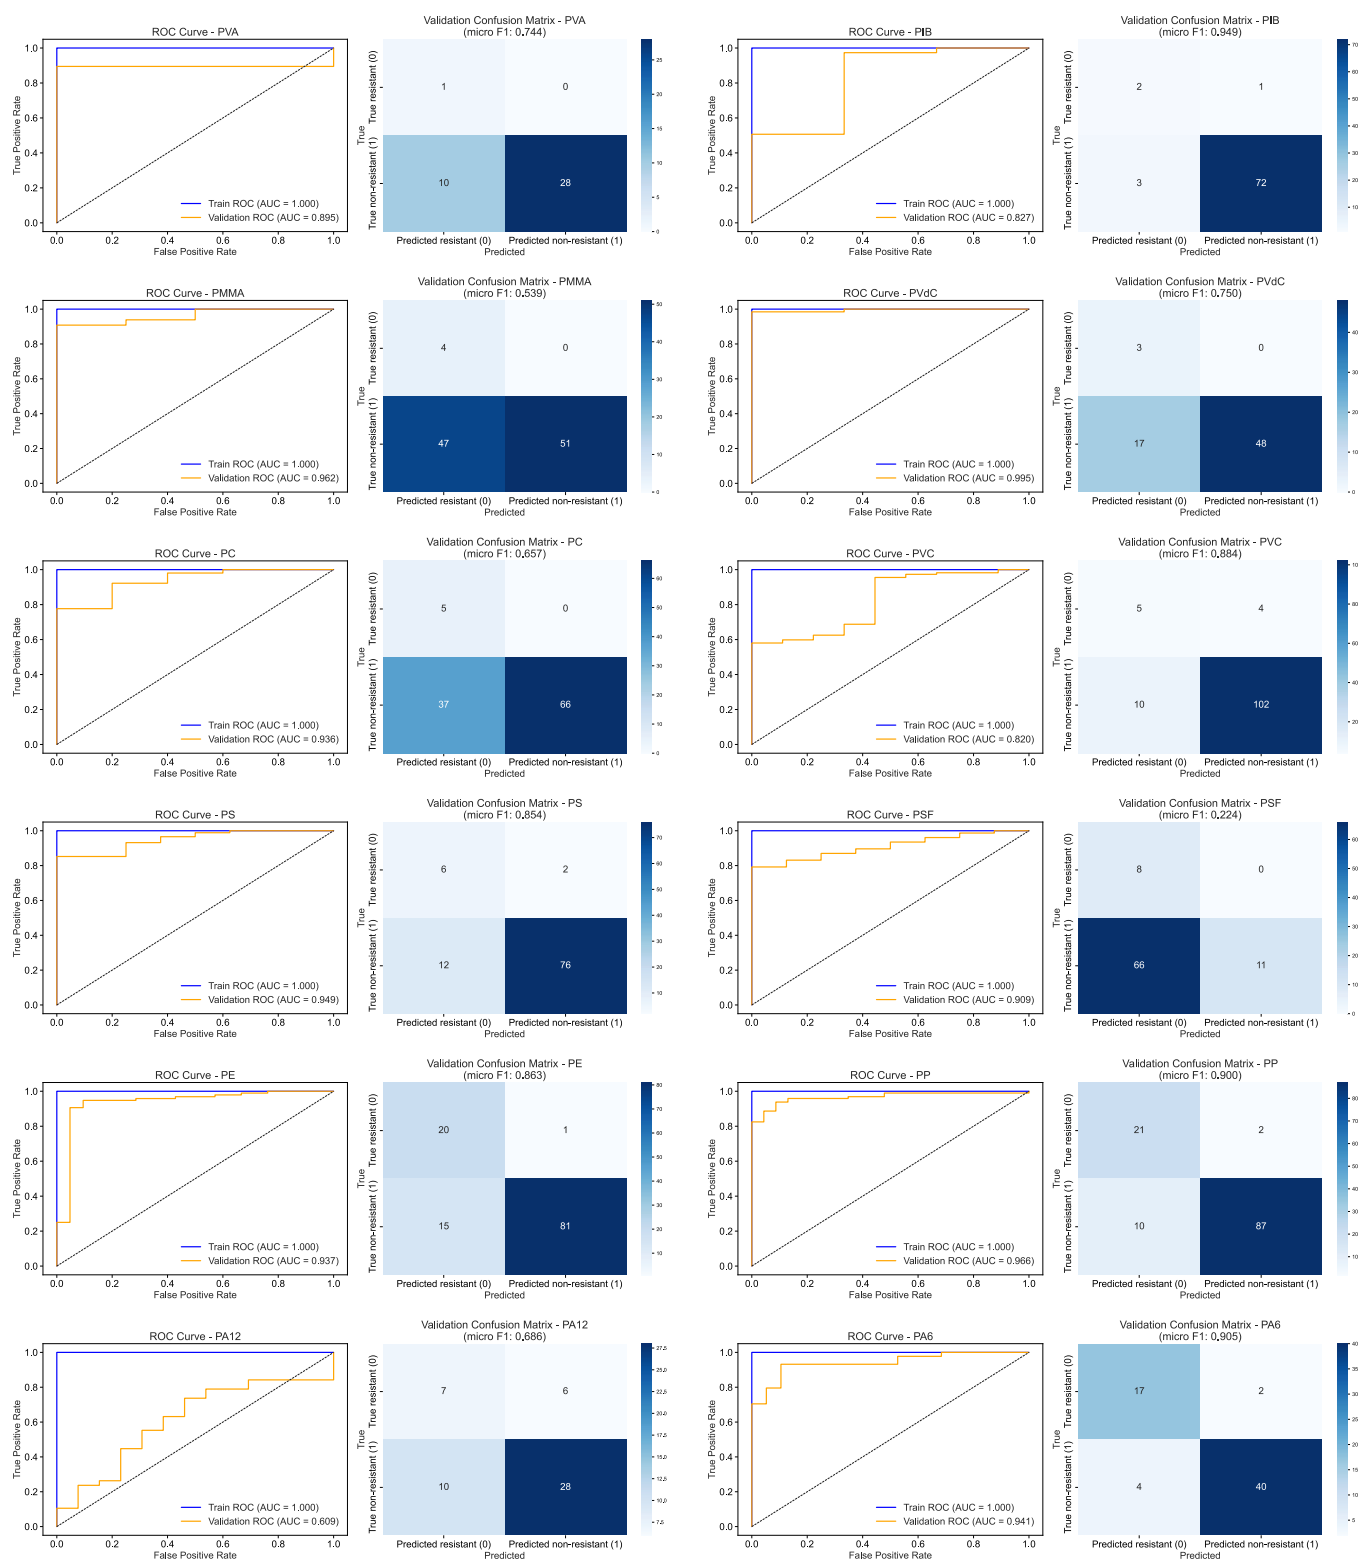

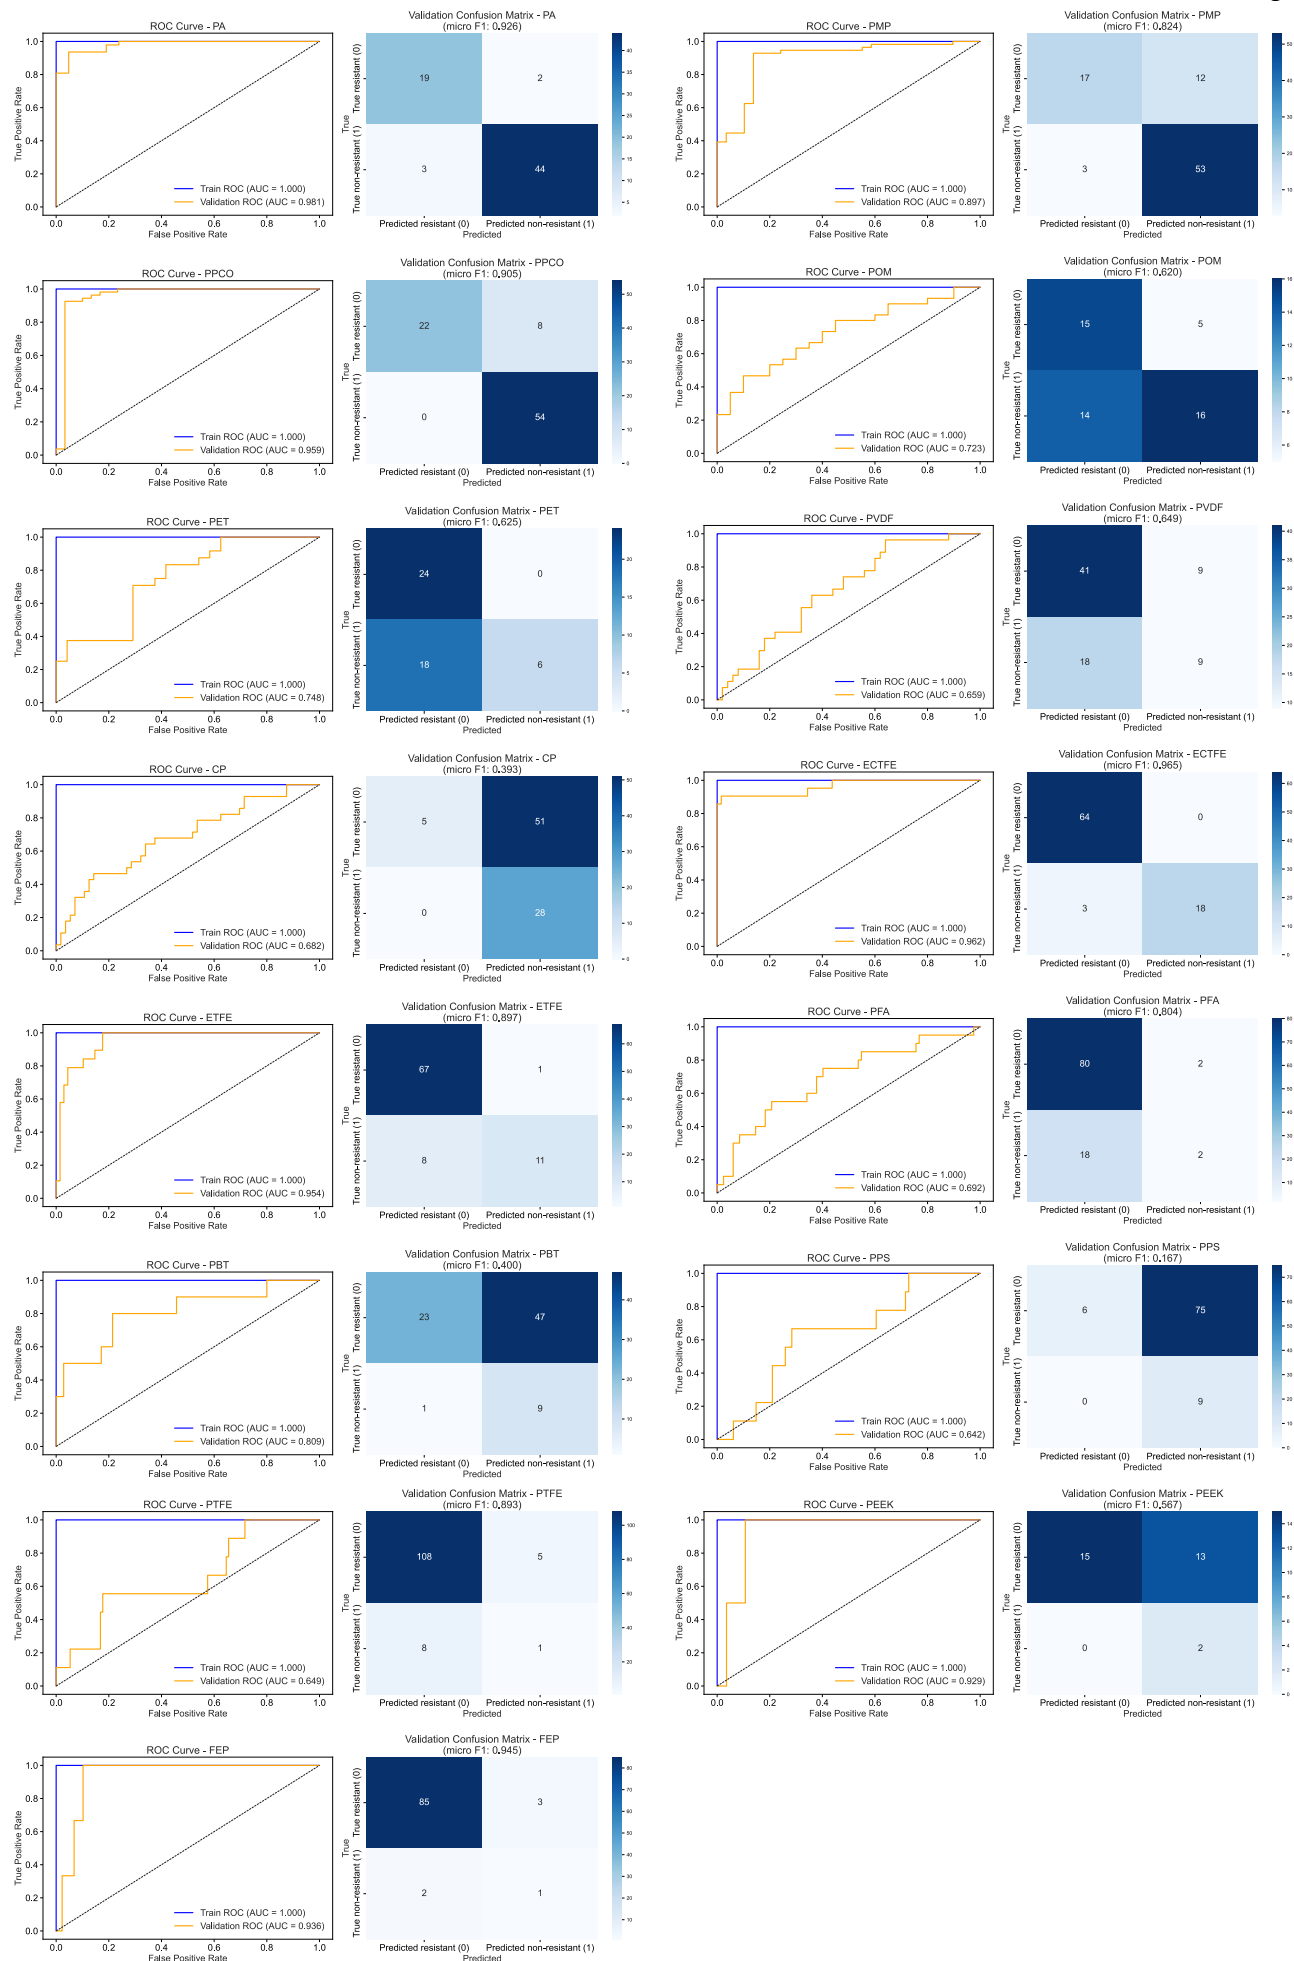

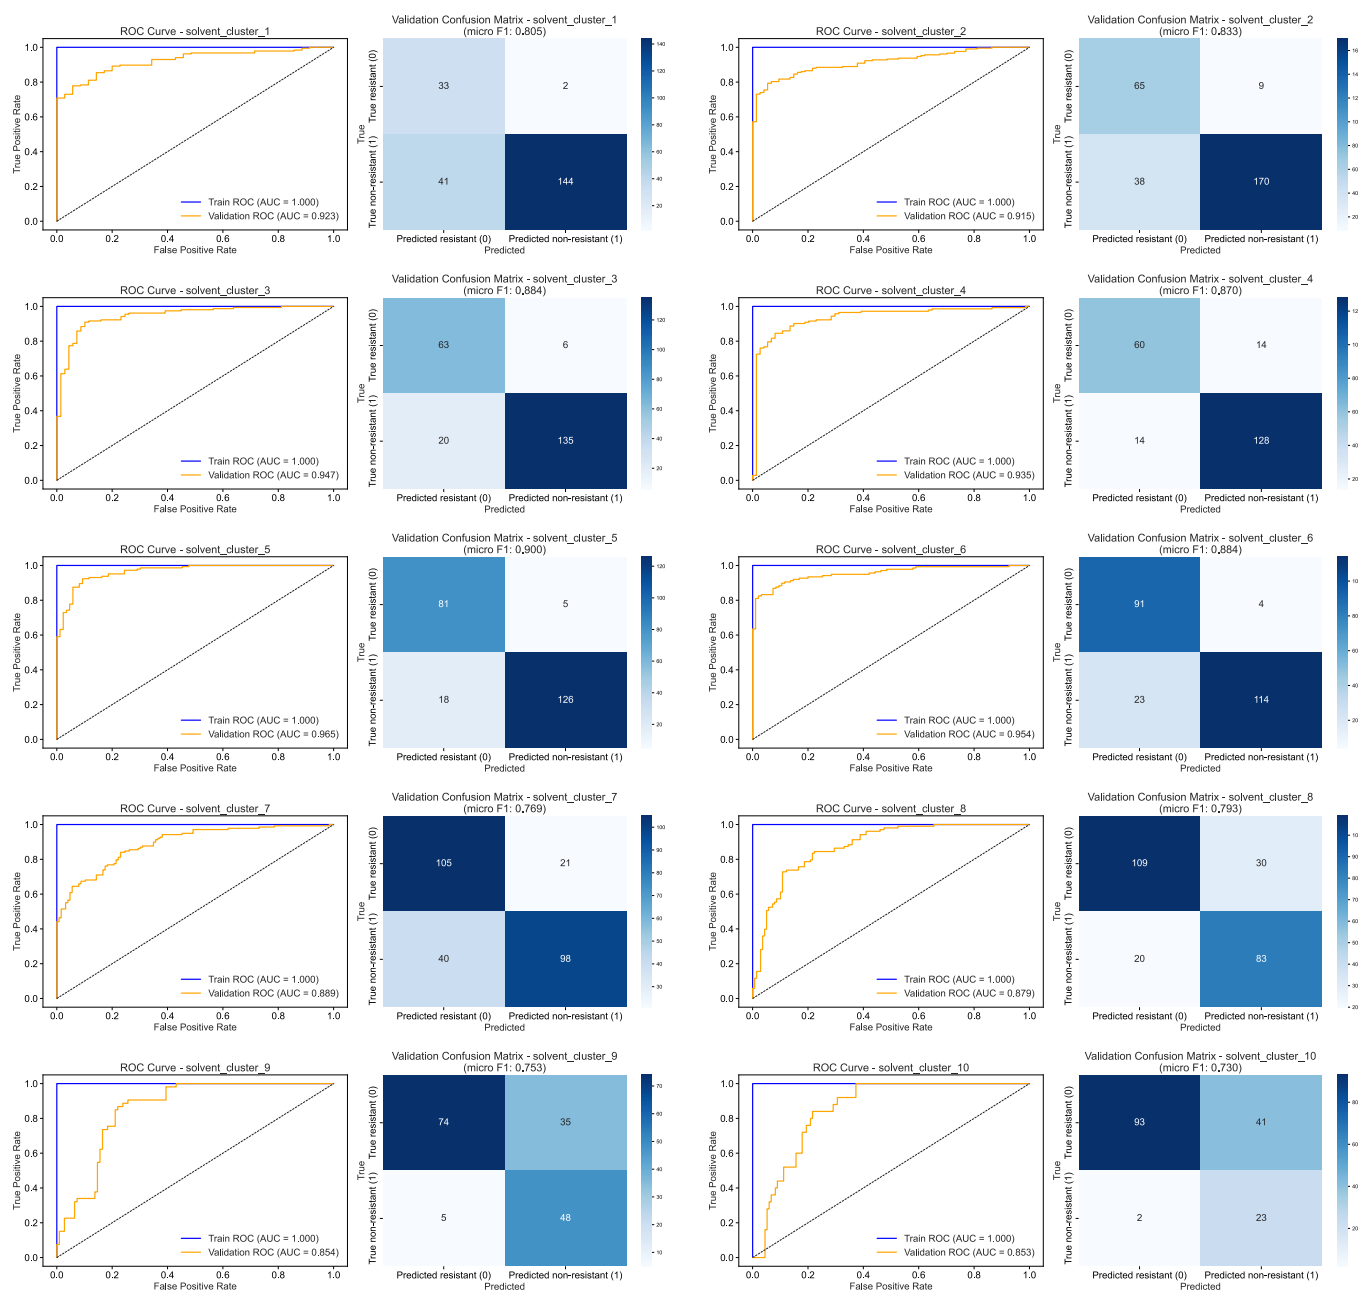

Figure S3: Leave-One-Group-Out Cross-Validation results for 27 polymers and 10 solvent clusters. For each polymer and solvent cluster, the left panel shows the ROC-AUC curves, with training and validation results shown in blue and orange, respectively. The right panel displays the confusion matrix for the validation results.

## 5. Validation results of the crystallinity classification model

This section presents the validation performance of the polymer crystallinity classification model, as referenced in Section 3.2 of the main text. The model was developed using XGBoost to classify crystallinity based on a dataset of 27 polymers, consisting of 18 crystalline and 9 amorphous polymers. After performing 9-fold cross-validation with 100 different random seeds, the average F1 score and ROC-AUC were  $0.794 \pm 0.213$  and  $0.706 \pm 0.373$ , respectively.

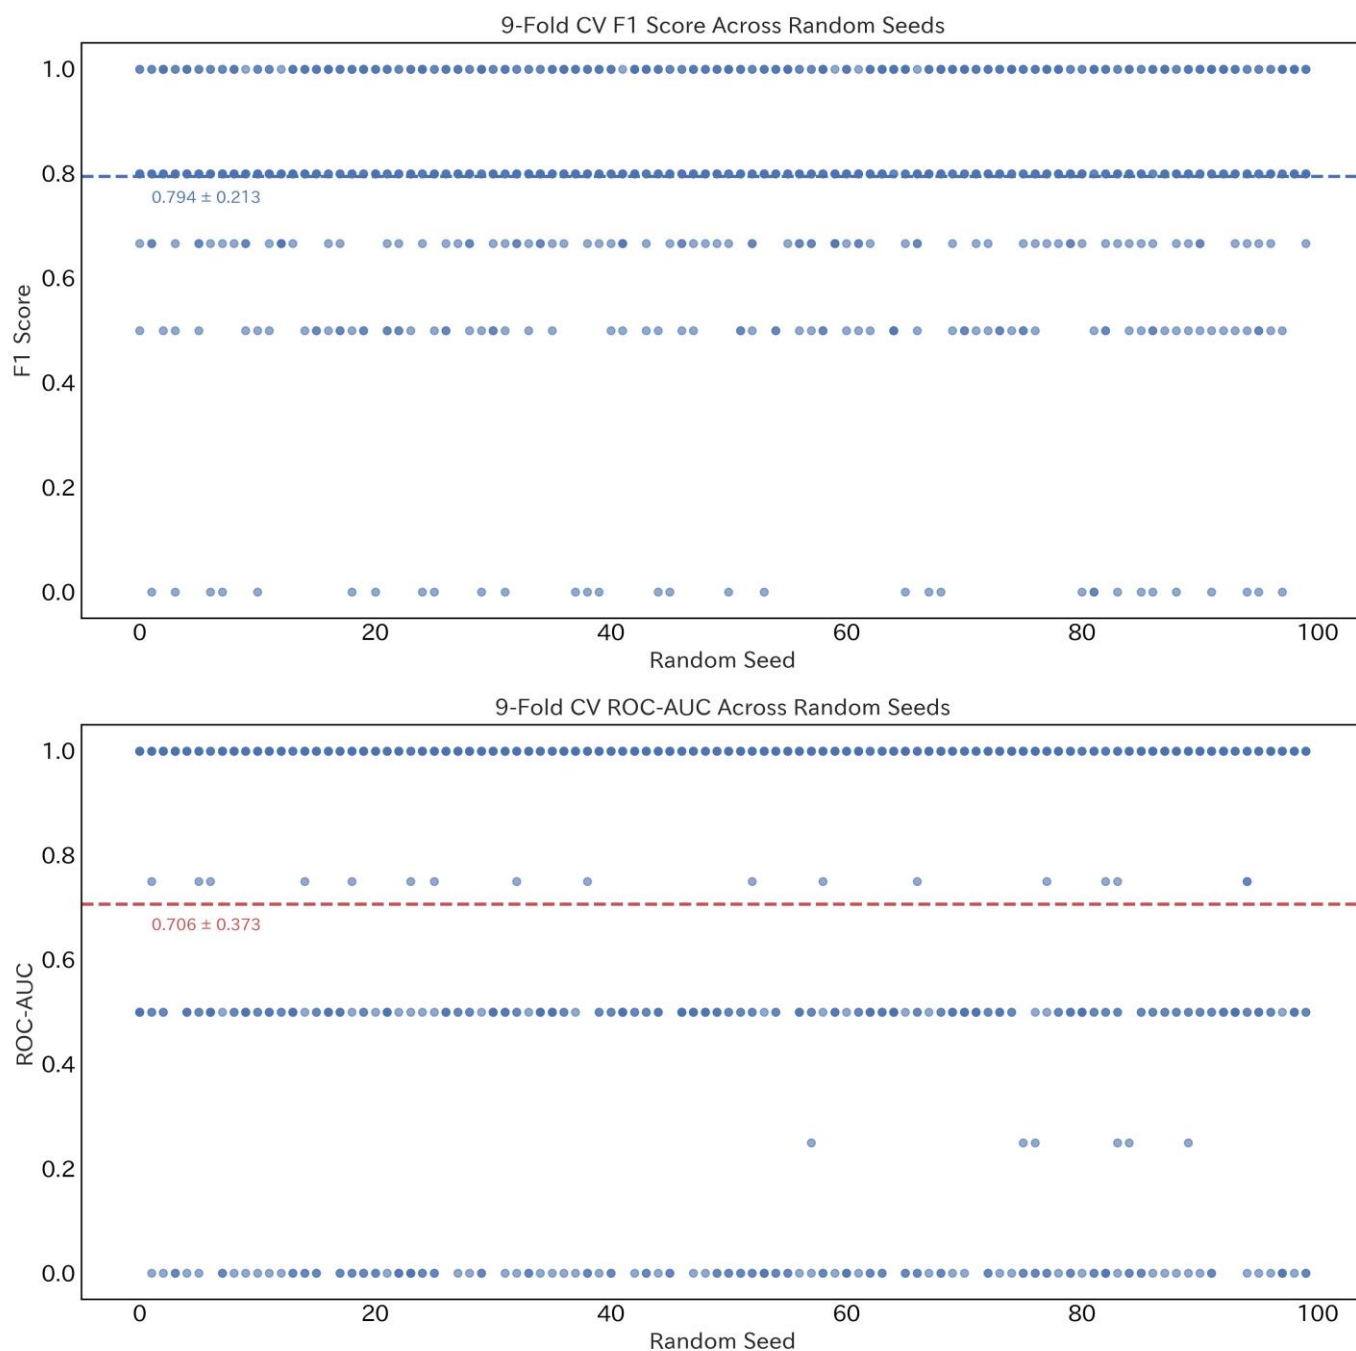

Figure S4: Validation performance of the classification model for crystallinity across 27 polymers.

(a) F1 score, (b) ROC-AUC. The x-axis represents different random seeds used for 9-fold cross-validation, and the y-axis shows the corresponding validation performance. Dashed lines indicate the average validation performance across all 100 trials.

## 6. Distribution of solvent properties

This section corresponds to the solvent feature analysis described in Section 3.4. Using the chemical resistance prediction model trained on 2,231 polymer–solvent data points, predictions were made for 9,828 virtual solvents against polyethylene (PE). Solvents with predicted chemical resistance probabilities greater than 0.9 are shown in red, representing highly soluble solvents, while those with predicted probabilities below 0.1 are shown in green, representing poorly soluble solvents.

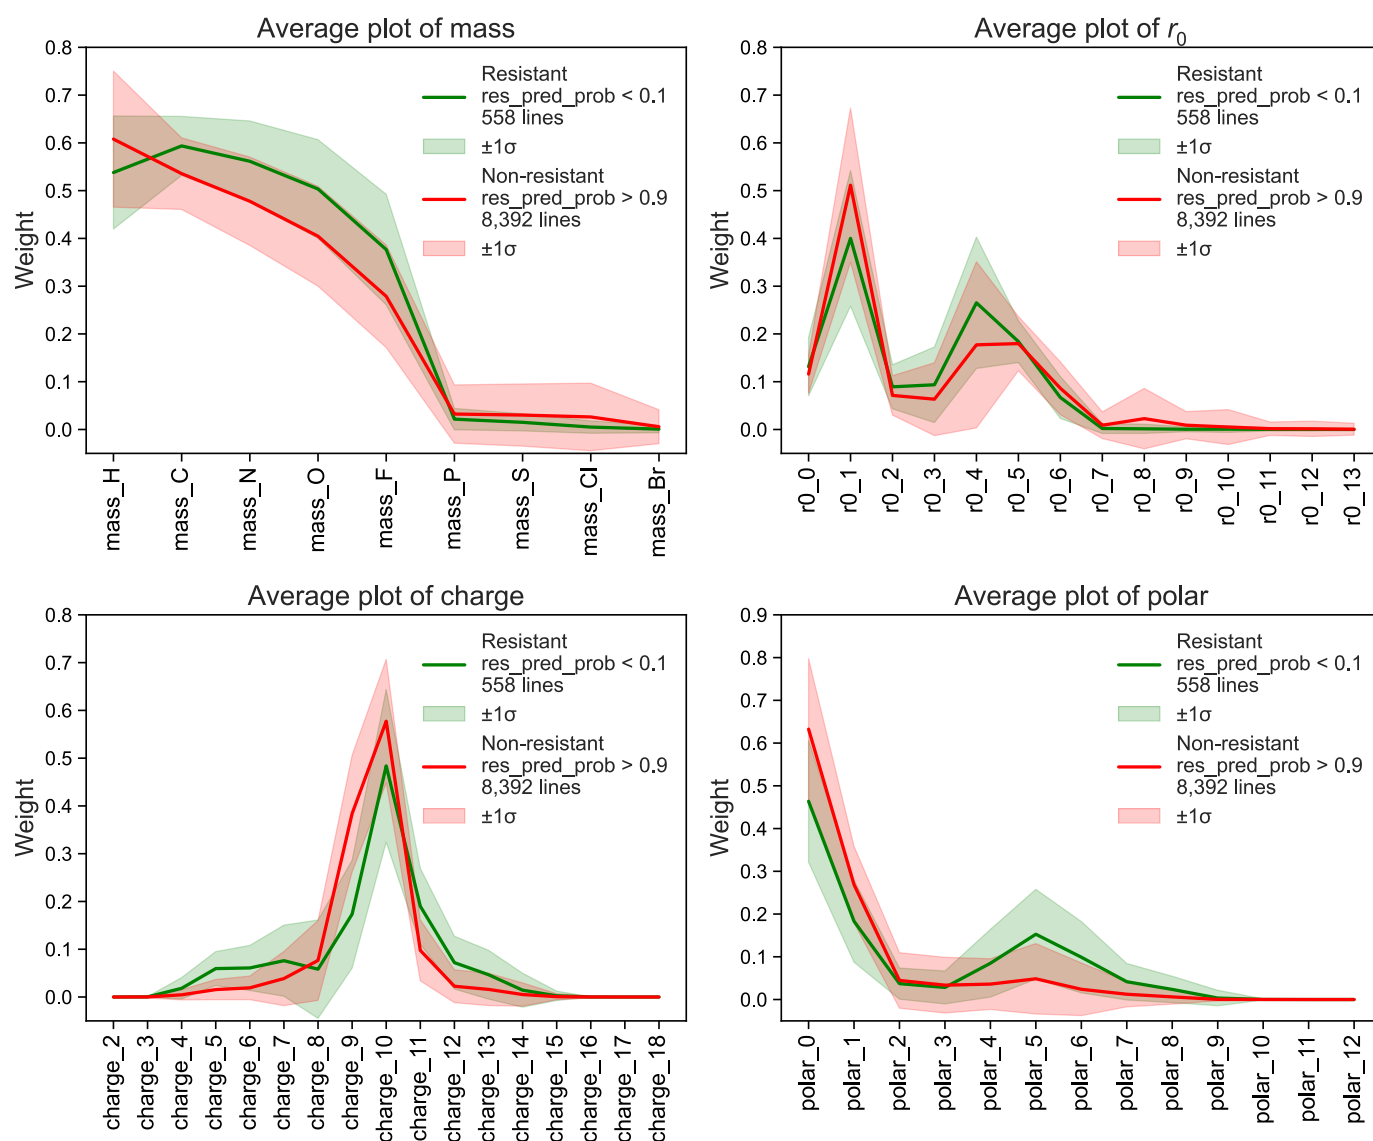

Figure S5: Feature analysis of organic solvents based on 10 FFKM parameters. The x-axis represents feature values, and the y-axis indicates probability density. Chemical resistance predictions were made for 9,828 virtual solvents against polyethylene (PE) using the chemical resistance prediction model. Solvents with predicted probabilities greater than 0.9 are shown in red (high solubility), and those with probabilities below 0.1 are shown in green (low solubility). For each group, the solid lines represent the mean values of the features, and the shaded areas indicate the standard deviations.

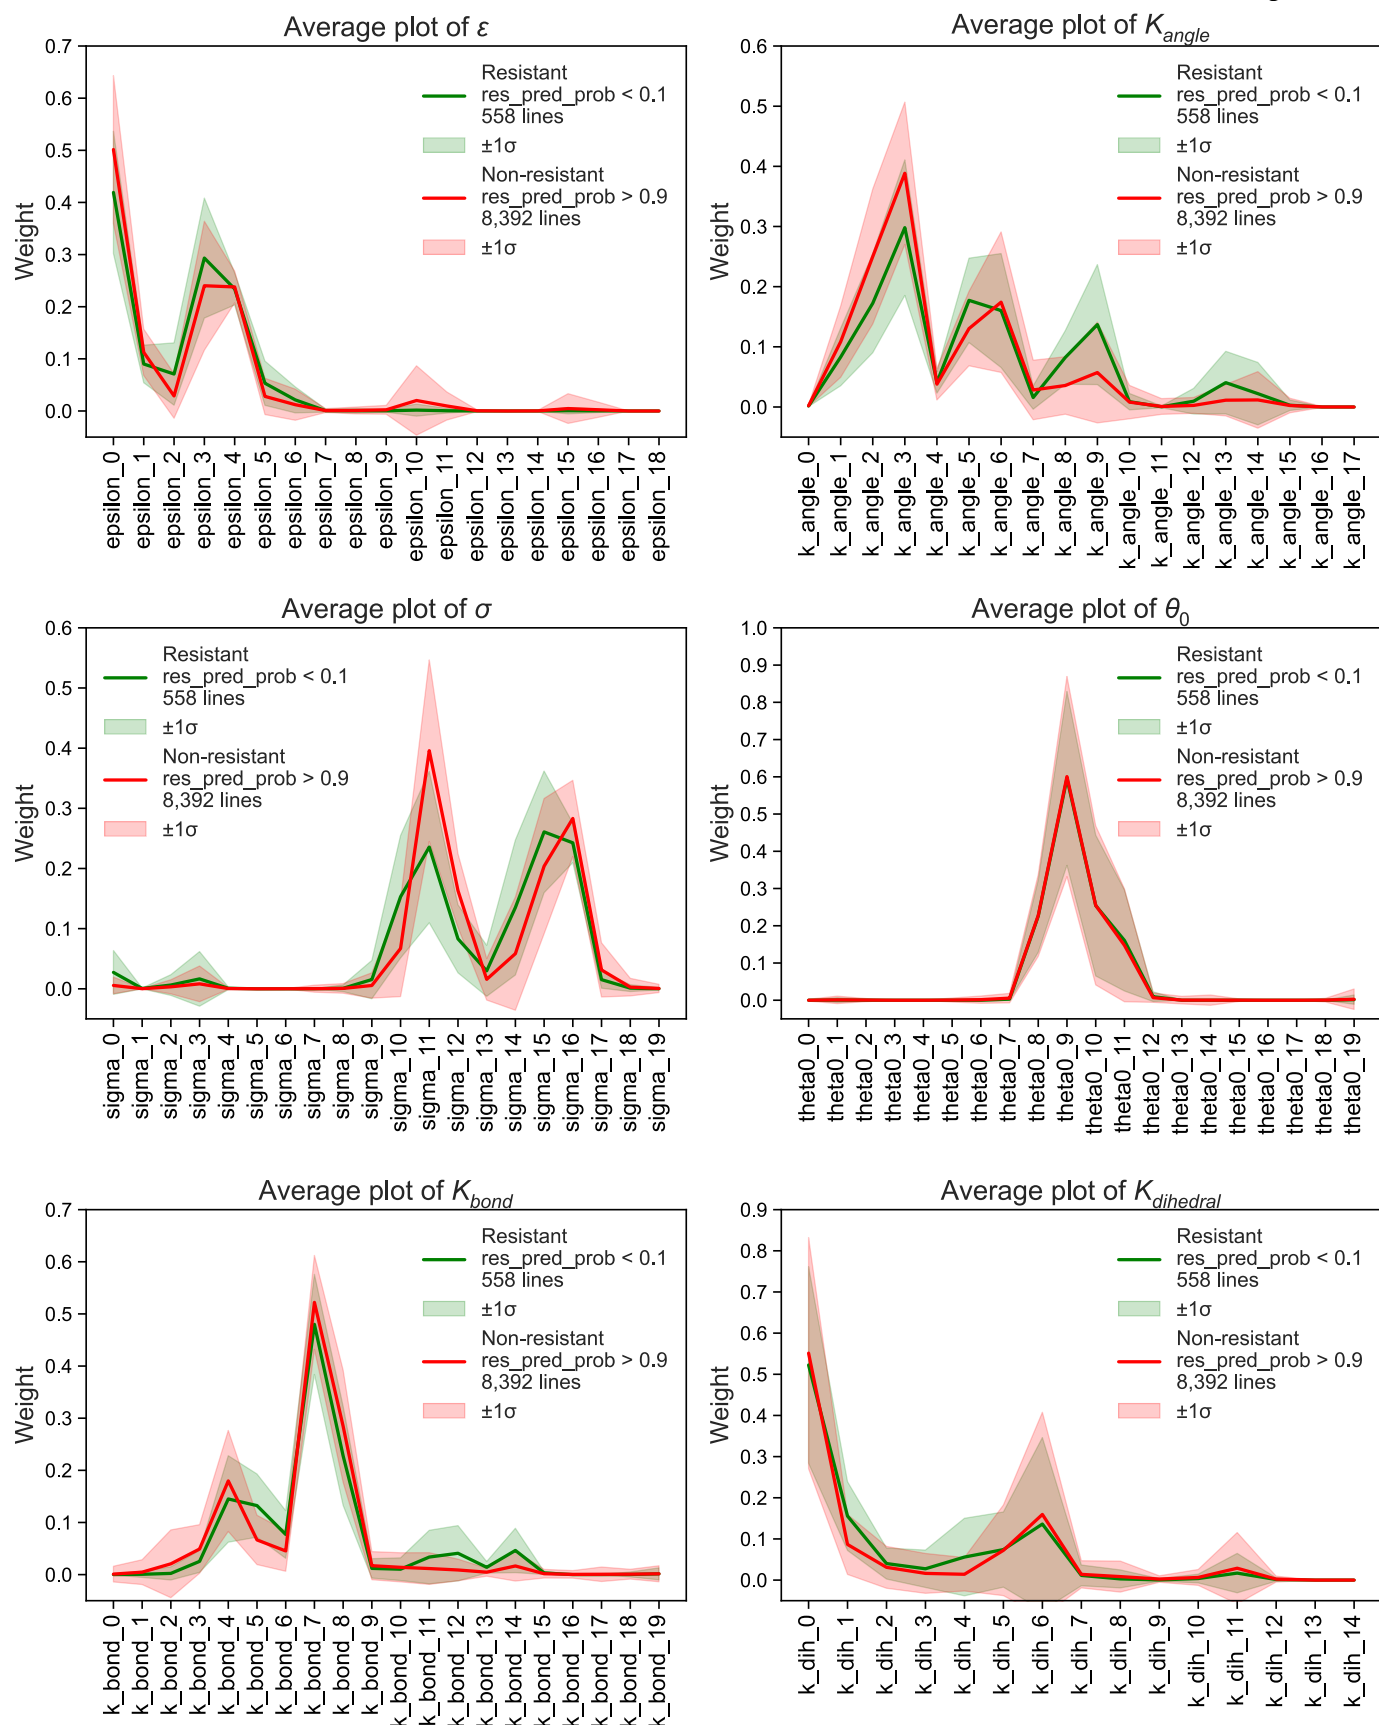

## 7. $\chi$ Parameter Distribution

Figure S6 presents histograms of the  $\chi$  parameters for the 27 polymers included in the chemical resistance dataset, calculated against 9,828 virtual solvents, as discussed in Section 3.5 of the main text. The distributions are stratified by chemical resistance classification (resistant vs. non-resistant) based on the predictions of the chemical resistance model.



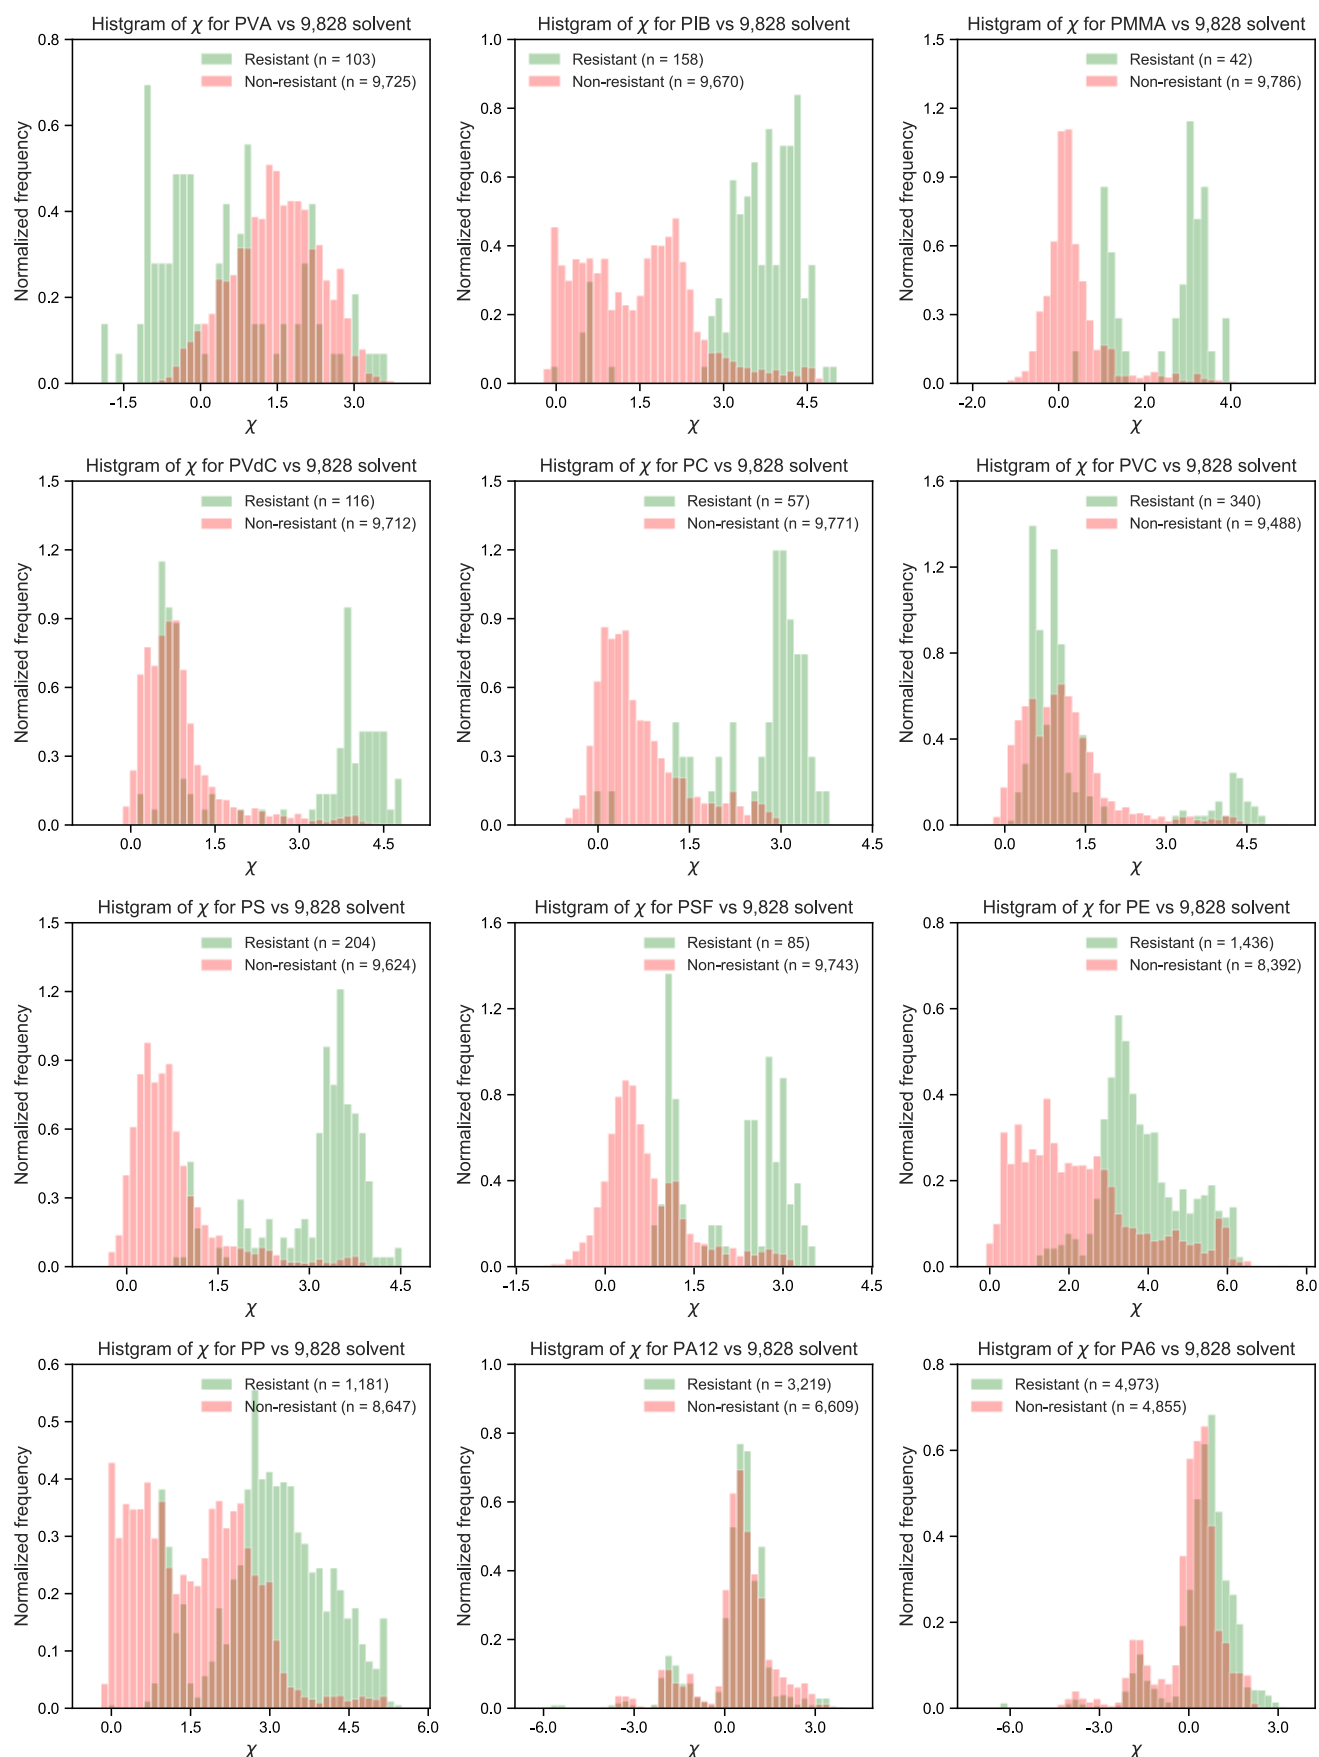

Figure S6: Histograms of  $\chi$  parameters for 27 polymers included in the chemical resistance dataset, calculated against 9,828 virtual solvents. The x-axis represents  $\chi$  values, and the y-axis shows the normalized data density. Chemical resistance classifications predicted by the model are color-coded: red for non-resistant and green for resistant.

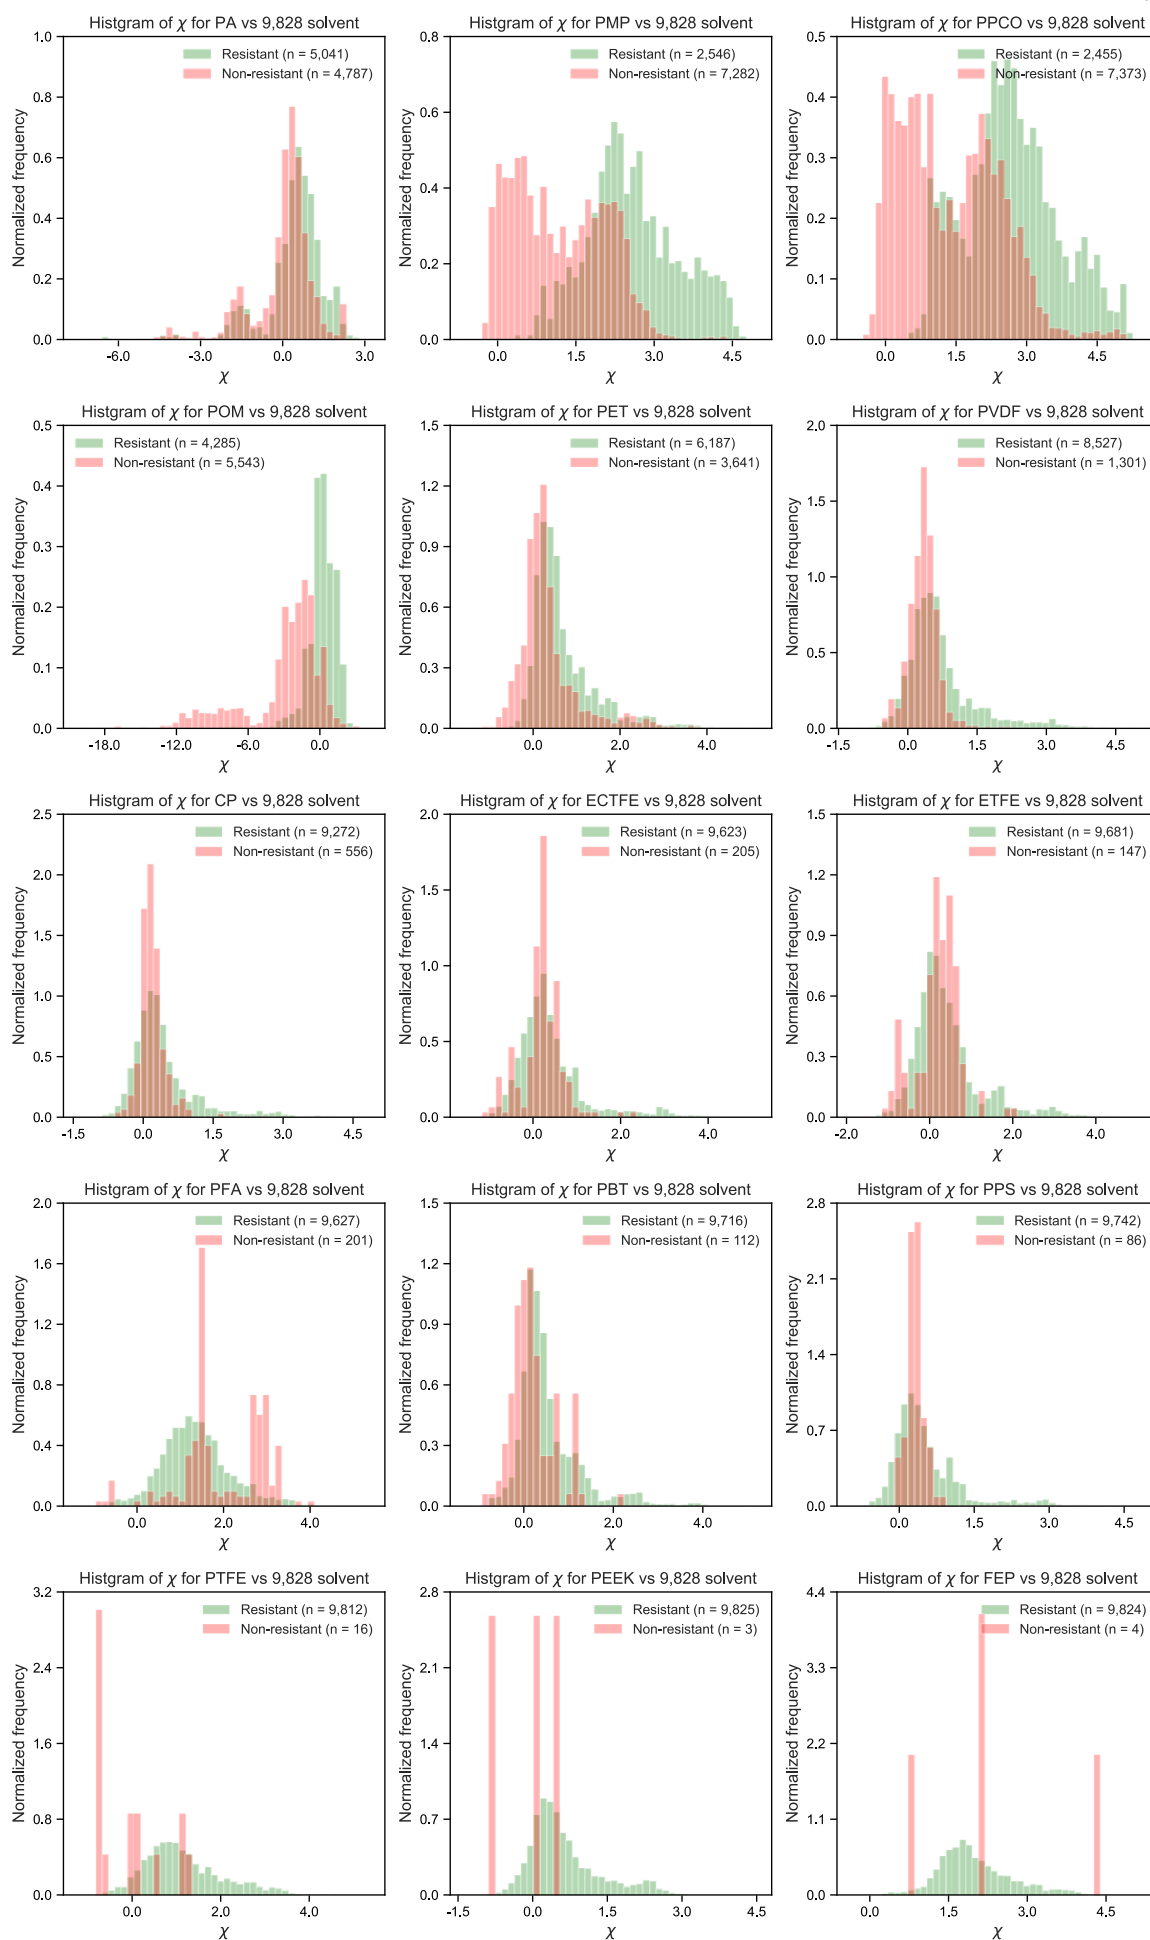

## 8. References

- (1) Chemical Resistance of Plastics: Oil, Solvent, and Chemical Resistance Chart, Kayo Corporation. [https://kayo-corp.co.jp/common/pdf/pla\\_proof.pdf](https://kayo-corp.co.jp/common/pdf/pla_proof.pdf).
- (2) *Chemical Resistance Chart, ASOH Co., Ltd.* <https://123deta.com/document/y4g9g49y-%E5%8C%96%E5%AD%A6%E8%96%AC%E5%93%81%E8%80%90%E6%80%A7%E8%A1%A8%EF%BD%9C%E3%82%A2%E3%82%BD%E3%83%BC%E6%A0%AA%E5%BC%8F%E4%BC%9A%E7%A4%BE.html> (accessed 2025-04-28).
- (3) *Chemical Resistance Data, PISCO Corporation.* <https://www.pisco.co.jp/technology/chemicalresistance/> (accessed 2025-04-28).
- (4) Chemical Resistance PEEK and Other Polymers, VICI AG International.
- (5) Chemical Resistance PCTFE, Professional Plastics.
- (6) Labware Chemical Resistance Table, Thermo Fisher Scientific.
- (7) Kusaba, M.; Hayashi, Y.; Liu, C.; Wakiuchi, A.; Yoshida, R. Representation of Materials by Kernel Mean Embedding. *Phys. Rev. B* **2023**, *108* (13), 134107. <https://doi.org/10.1103/PhysRevB.108.134107>.
- (8) RadonPy Github Site, 2025. <https://github.com/RadonPy/RadonPy> (accessed 2025-04-28).
- (9) *TURBOMOLE | Program Package for Electronic Structure Calculations.* TURBOMOLE. <https://www.turbomole.org/> (accessed 2025-04-28).
- (10) Eckert, F.; Weg, I. COSMOtherm, Version C3.0, Release 17.01; COSMOlogic GmbH & Co. KG, [Http://Www.Cosmologic.De](http://www.Cosmologic.De).
- (11) Aoki, Y.; Wu, S.; Tsurimoto, T.; Hayashi, Y.; Minami, S.; Tadamichi, O.; Shiratori, K.; Yoshida, R. Multitask Machine Learning to Predict Polymer–Solvent Miscibility Using Flory–Huggins Interaction Parameters. *Macromolecules* **2023**, *56* (14), 5446–5456. <https://doi.org/10.1021/acs.macromol.2c02600>.
